# Supplementary material for: Low temperature synthesis of BiFeO$_{3}$ nanoparticles with enhanced magnetization and promising photocatalytic performance in dye degradation and hydrogen evolution
Source: arXiv:2202.02505 source file (2022-02-05)
Supplement: Supplementary file 1 [file appendix1.tex]

\section{Supplementary Material} \label{sec:appendix}
    Here the ESI will be included.
